# Supplementary material for: Clustering free-falling paper motion with complexity and entropy
Source: arXiv:2204.14097 source file (2022-04-29)
Supplement: Supplementary file 1 [file supplementary.pdf]

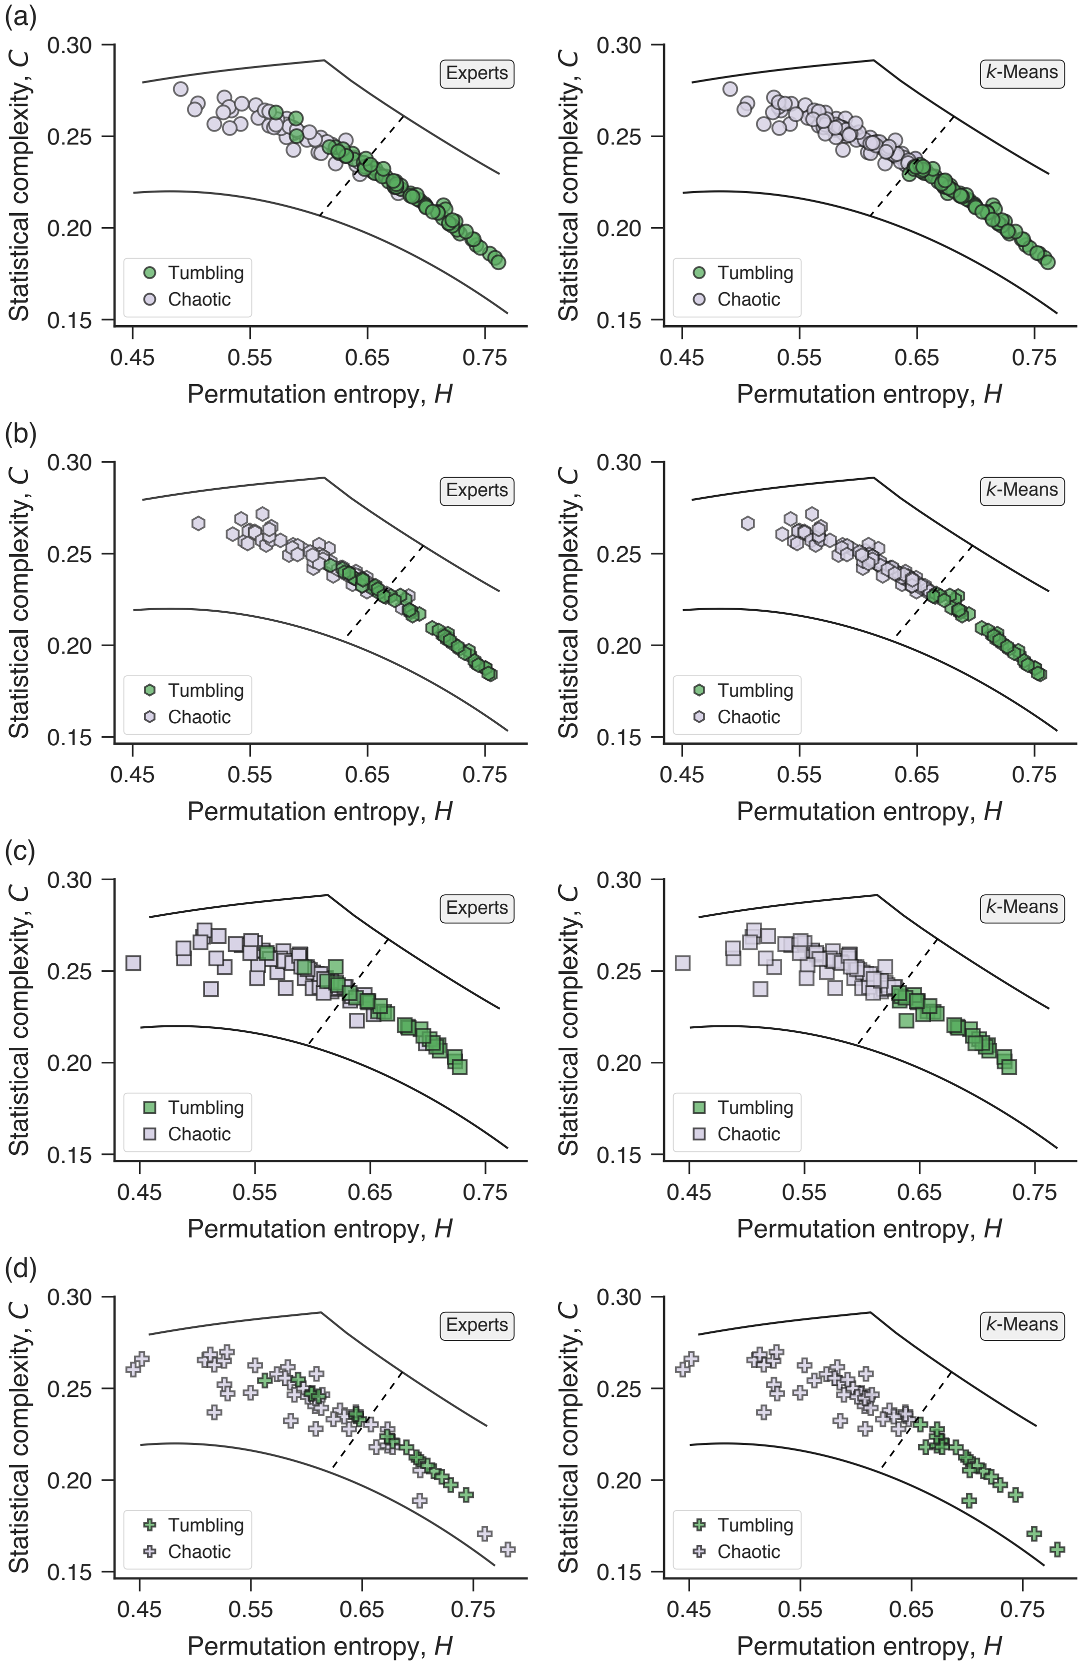


Fig. 1: Panels (a) to (d) show the complexity-entropy plane obtained from time series of the observable area of paper sheets with circle, hexagon, square, and cross shapes, respectively. Plots in the left column represent the classification made by a panel of human experts, while those on the right show the automatic classification obtained by applying the $k$-means algorithm (with $k = 2$ groups) to the entropy and complexity values. In all panels, the continuous curves indicate the minimum and maximum complexity values for a given value of entropy, while the dashed lines represent the decision boundary obtained from the $k$-means algorithm.

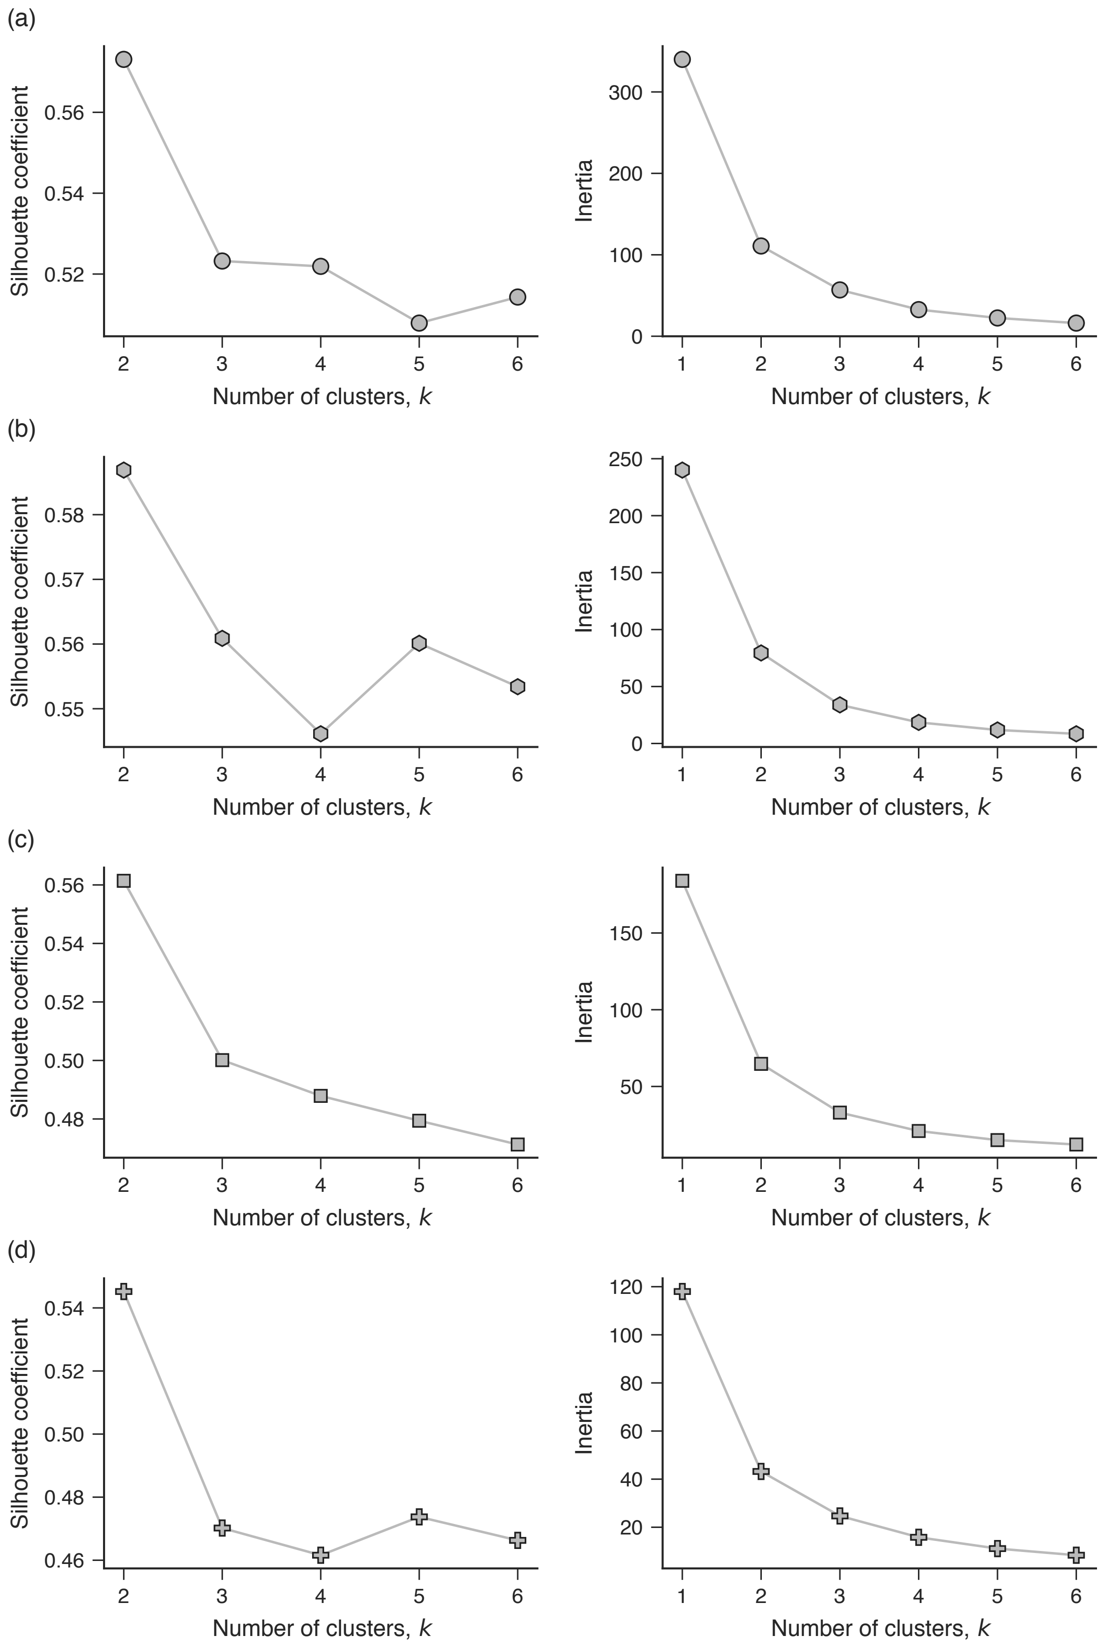


Fig. 2: Silhouette score (plots on the left column) and cluster inertia (plots on the right column) for different values of $k$ (number of groups). Panels (a) to (d) show the results for clustering the time series related to paper sheets with circle, hexagon, square, and cross shapes, respectively. We observe that $k = 2$ yields the best partition according to silhouette score and the "elbow method" with the cluster inertia (within-cluster sum-of-squares).
